# Supplementary material for: SOLVE: Synergy of Language-Vision and End-to-End Networks for Autonomous Driving
Source: arXiv:2505.16805 source file (2025-05-22)
Supplement: Supplementary file 1 [file X_suppl.tex]

\clearpage
\setcounter{page}{1}
\maketitlesupplementary

\suppsection{Additional details of the SQ-Former}
To effectively encode diverse visual information, we propose the SQ-Former architecture, which implements sequential feature collection and alignment through perception queries. As shown in Figure 3 in the main paper, SQ-Former introduces collector queries as visual information carriers, which sequentially accumulate information from global image features, 3D object detection, and lane detection queries through attention mechanisms.

For multi-view image features, collector queries interact with them through 6 transformer layers, with each layer comprising a self-attention and a cross-attention operation. This interaction enables the collector queries to extract background contextual information, including environmental conditions, time of day, etc., that not presented in detection or lane queries.
Following the acquisition of scene-level information, the collector queries are concatenated with detection queries and processed through the detection decoder to extract foreground object information, as shown in Figure~\ref{fig:decoder}. Following StreamPETR~\cite{wang2023exploring}, the detection decoder employs two types of queries: initial queries, which are learned from current frame data to detect newly appearing objects, and temporal queries, which are propagated from last frames to maintain object tracking continuity.
In the concatenation of collector queries with temporal and initial queries, we implement an asymmetric attention mask, which enables unidirectional information flow from detection queries to collector queries while prevents the flow in the opposite direction. The asymmetric design ensures that the collector query can effectively obtain information from the detection query without affecting the performance of the detector.

Through temporal attention, collectors can acquire historical motion information from temporal queries and initial queries can identify previously tracked objects to focus on new detections in the current frame. The subsequent cross attention operation allows temporal queries to verify the persistence of tracked objects, while initial queries identify new object instances. 
Through multiple iterations of this process, collector queries develop a comprehensive understanding of foreground objects within the current scene. Meanwhile, the temporal query and the initial query can detect the tracked objects and the newly appeared objects well, and then the topK operation selects these queries by confidence and places them into the memory queue.

The architecture of lane decoder is similar to that of detection decoder, except that the temporal query is not used, as shown in Figure~\ref{fig:decoder}. After interacting with the lane query, the collector query can understand the road structure of the current scene, which is useful for trajectory planning.

For hyper-parameter settings, we use 6 transformer layers (including temporal attention and cross attention), 900 initial queries, 300 temporal queries (equal to the selection number of topk operation), and the length of the memory bank is two frames (600 queries) for the detection decoder. For the lane decoder, we also use 6 transformer layers, 300 initial queries, and the length of the memory bank is two frames (600 queries). The number of collector queries is 384 and all queries with the channel number of 256.

% This sequential architecture ensures efficient information integration and robust scene understanding through specialized query interactions and attention mechanisms.

\begin{figure}[!t]
\centering
\includegraphics[width=0.49\textwidth ]{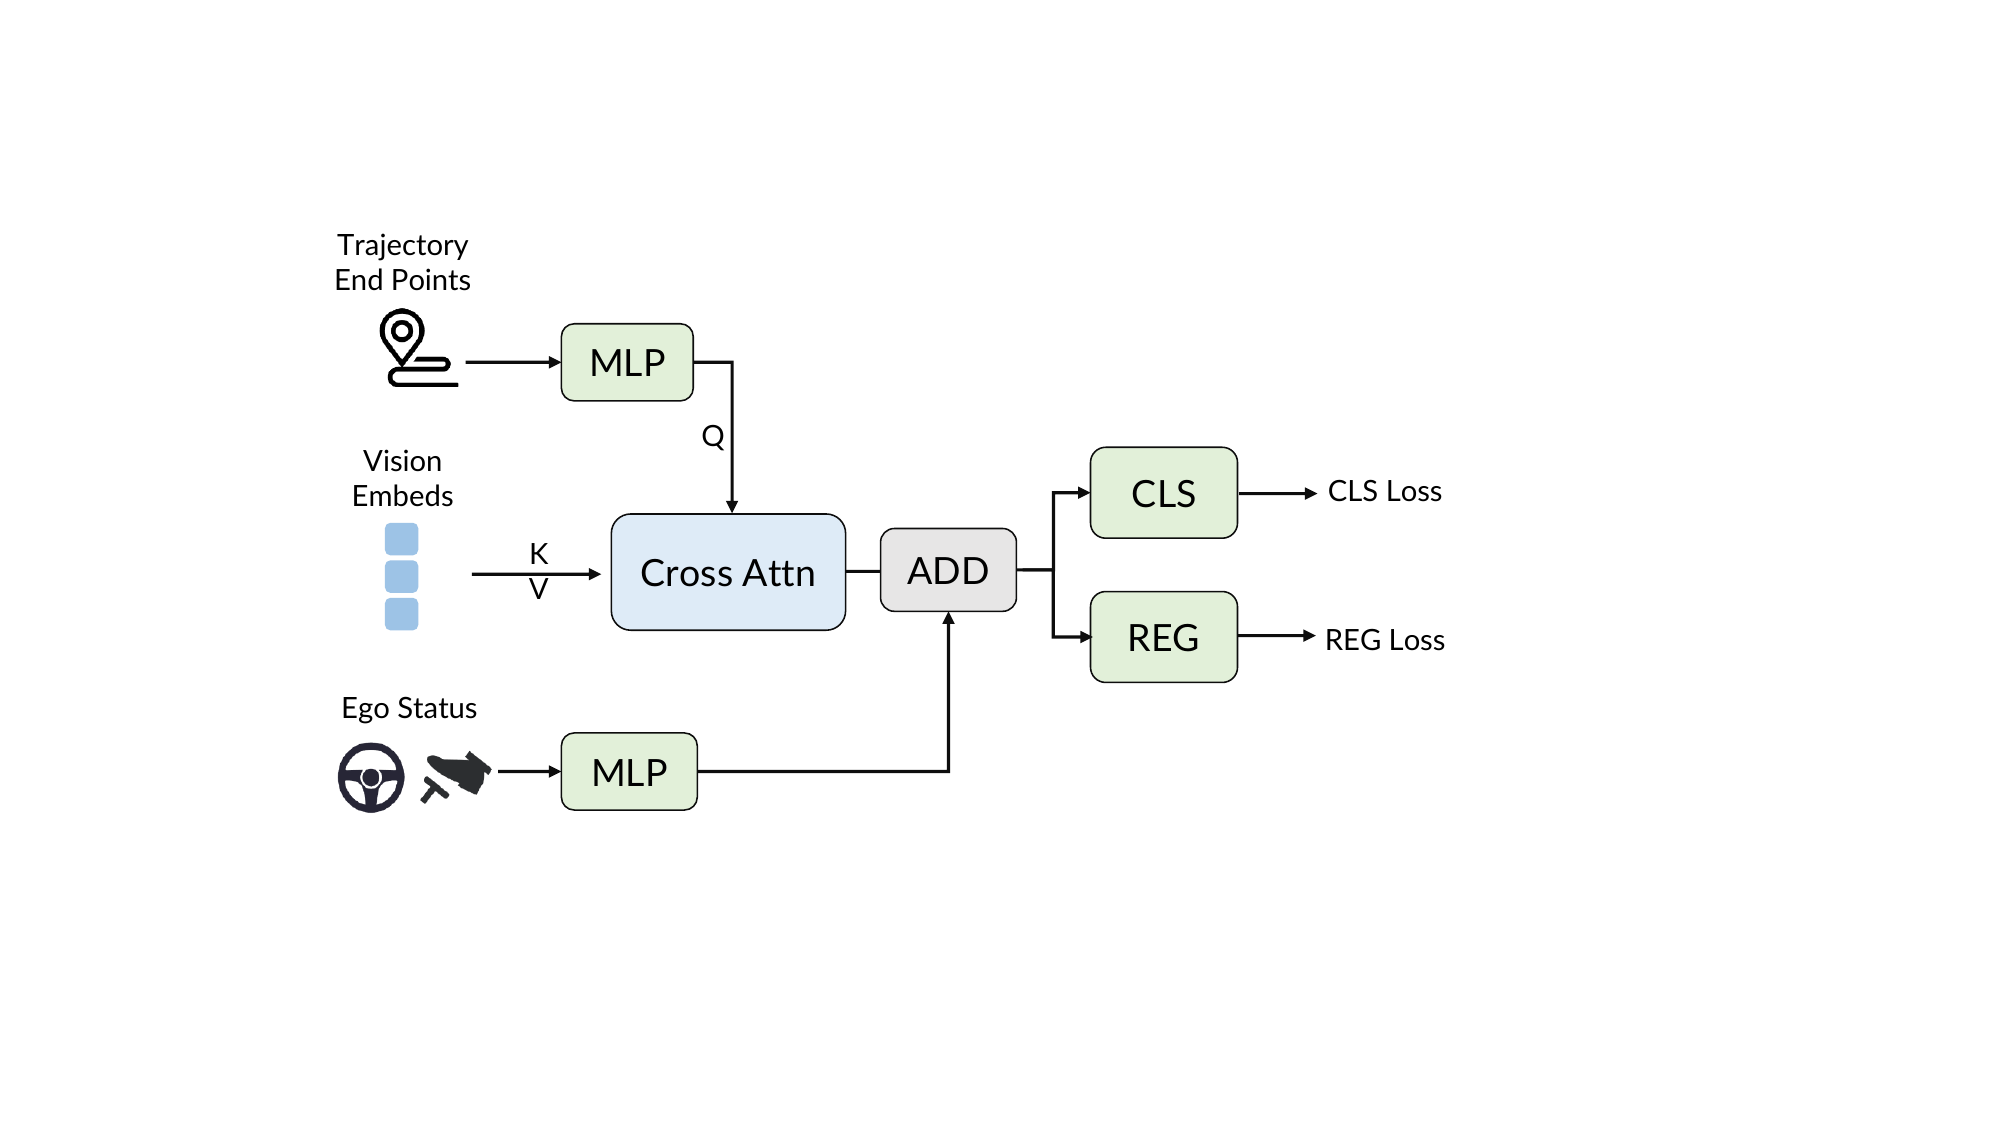}
\caption{Detail design of the End-to-end (E2E) planner of SOLVE. Ego status includes the speed, acceleration, and angular velocity of the ego car in current scene. Vision Embeds are the shared collector queries.}
\label{fig:e2e}
\end{figure}

\begin{figure*}[!t]
\centering
\includegraphics[width=0.99\textwidth ]{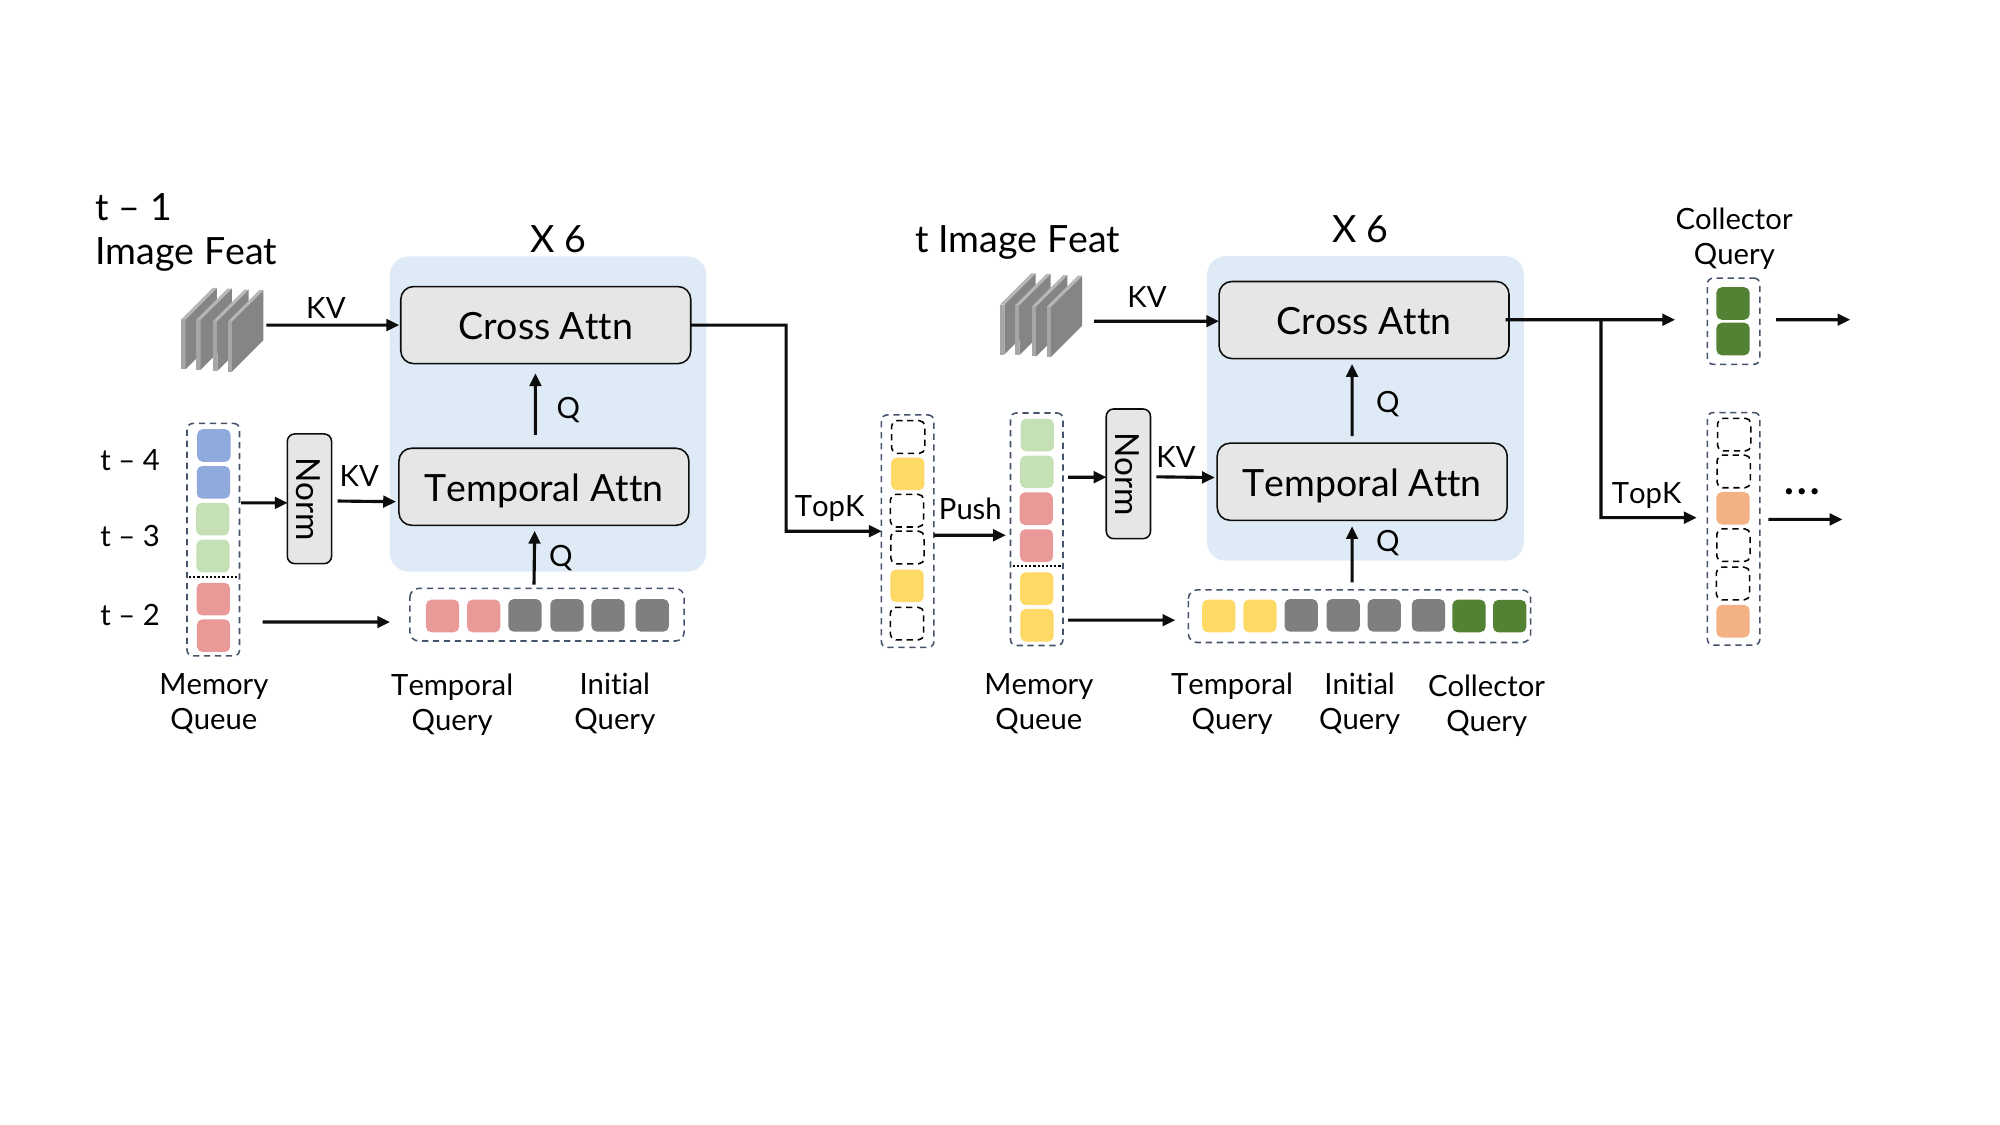}
\caption{Illustration of the temporal detection and lane decoder in our proposed SQ-Former. Note that temporal queries are \textbf{only} used in the detection decoder, where each temporal query represents a tracked object. For each frame, the collector query obtains information about foreground objects and road structures in the scene by interacting with the initial query and propagated temporal query (only for detection) at the current moment. At the same time, the collector query can obtain long-term temporal context information by interacting with the historical queries in the memory bank.}
\label{fig:decoder}
\end{figure*}

\suppsection{Additional details of the End-to-end planner}
As shown in the Figure~\ref{fig:e2e}, we propose an efficient end-to-end planning architecture that employs a discrete set of 18 predefined trajectories, categorized into three motion primitives: forward, left-turn, and right-turn, with six variants per category. In practice, we use the kmeans algorithm to cluster trajectories of the training dataset to obtain these 18 predefined trajectories. The trajectory endpoints are encoded via MLP into position embeddings to form planning queries.  These planning queries interact with collector queries (vision embedding) extracted from SQ-Former through two cross-attention layers. Finally, the classification head and regression head based on MLP are used to obtain the classification score and predicted trajectory of the planning query added with the ego embedding , respectively. We select the trajectory with the highest score as the final planning result. All queries with 256 channel.

\suppsection{Additional details of the training losses}
The training loss of SOLVE mainly consists of three parts, $L_{sqformer}$, $L_{vlm}$, $L_{e2e}$. Specifically, $L_{sqformer}$, which is used to supervise object detection and lane detection for the corresponding query in SQ-Former, includes $L_{det}$ and $L_{lane}$. For $L_{vlm}$, we use cross entropy loss to supervise the next token prediction of auto-regression and we adopt a loss weight that sets number (0$\sim$9) and signs $\pm$ to 5 for more accurate digital prediction in trajectory planning. For $L_{e2e}$, following SparseDrive, we use cross entropy as classification loss and L2 loss as regression loss.
Finally, the total loss $L$ is expressed as: 
\begin{equation}
\mathcal{L}= \mathcal{L}_{\mathrm{sqformer}} + \mathcal{L}_{\mathrm{vlm}} + \mathcal{L}_{\mathrm{e2e}}.
\label{eq:loss}
\end{equation}

\begin{table}[t!]
\centering
\scalebox{0.9}{
\begin{tabular}{l|l|c|c}
\toprule
Planner & Method            & L2 (cm) & FPS \\ \hline \hline
\multirow{4}{*}{E2E} & $\text{UniAD}^*$~\cite{hu2023planning} (Res101) & 103.0   & 1.8 \\
& VAD~\cite{jiang2023vad} (Res50)          & 37.0    & 5.6 \\
& SOLVE-E2E (Res50) & 31.3    & 9.1 \\
& SOLVE-E2E (EVA-L) & 31.0    & 2.0 \\ \hline \hline
\multirow{3}{*}{VLM} & Omnidrive~\cite{wang2024omnidrive} (EVA-L)         & 33.0    & 0.3   \\
& SOLVE-VLM (Res50) & 29.9    & 0.3   \\
& SOLVE-VLM (EVA-L) & 28.4    & 0.3   \\
\bottomrule
\end{tabular}
}
\caption{Comparison of different method’s inference time and the adopted image backbone is indicated in brackets. All
methods are evaluated on NVIDIA A100 GPU. $*$ means ego status are not used in trajectory planning. }
\label{tab:time}
\end{table}

\suppsection{Additional analysis of inference time}
Table~\ref{tab:time} presents a comparison of performance and inference speed between end-to-end planners and VLM-based planners. The results indicate that VLM-based planners achieve superior performance, while End-to-end planners exhibit notable advantages in computational efficiency. Specifically, for the end-to-end planner, SOLVE-E2E (Res50) achieves the best efficiency and outperforms VAD by 5.7 in terms of L2 (cm). On the other hand, SOLVE-E2E (EVA-L) achieves the best performance with a more computationally expensive backbone. For the VLM planner, both with the res50-based lightweight image backbone and the EVA-L-based large backbone, SOLVE-VLM achieves higher performance than Omnidrive and E2E models.
